# Supplementary material for: Imperfect Visual Verification for Code Edition : A Case Study on TikZ
Source: arXiv:2606.15693 source file (2026-04-09)
Supplement: Supplementary file 1 [file additional_figures.tex]

\begin{figure*}
    \centering
    \includegraphics[width=\linewidth]{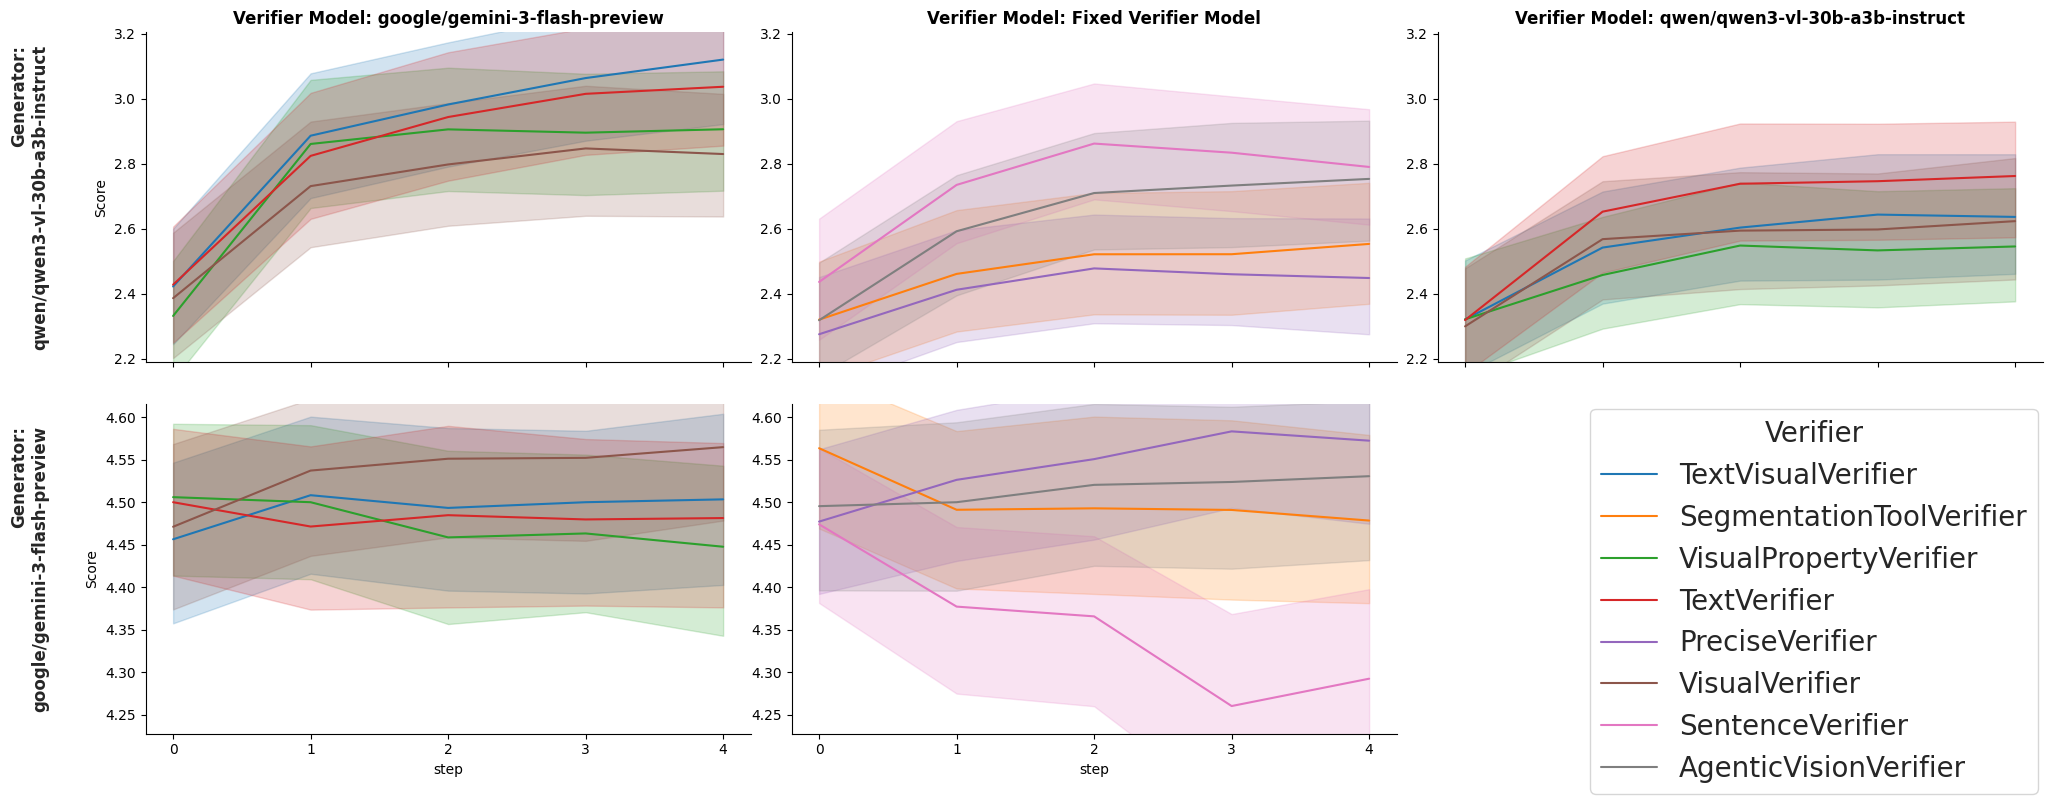}
   \caption{
       Average human score per step per Verifier.
   }
    \label{figure:avg_score_step}
\end{figure*}

\begin{figure*}
    \centering
    \includegraphics[width=\linewidth]{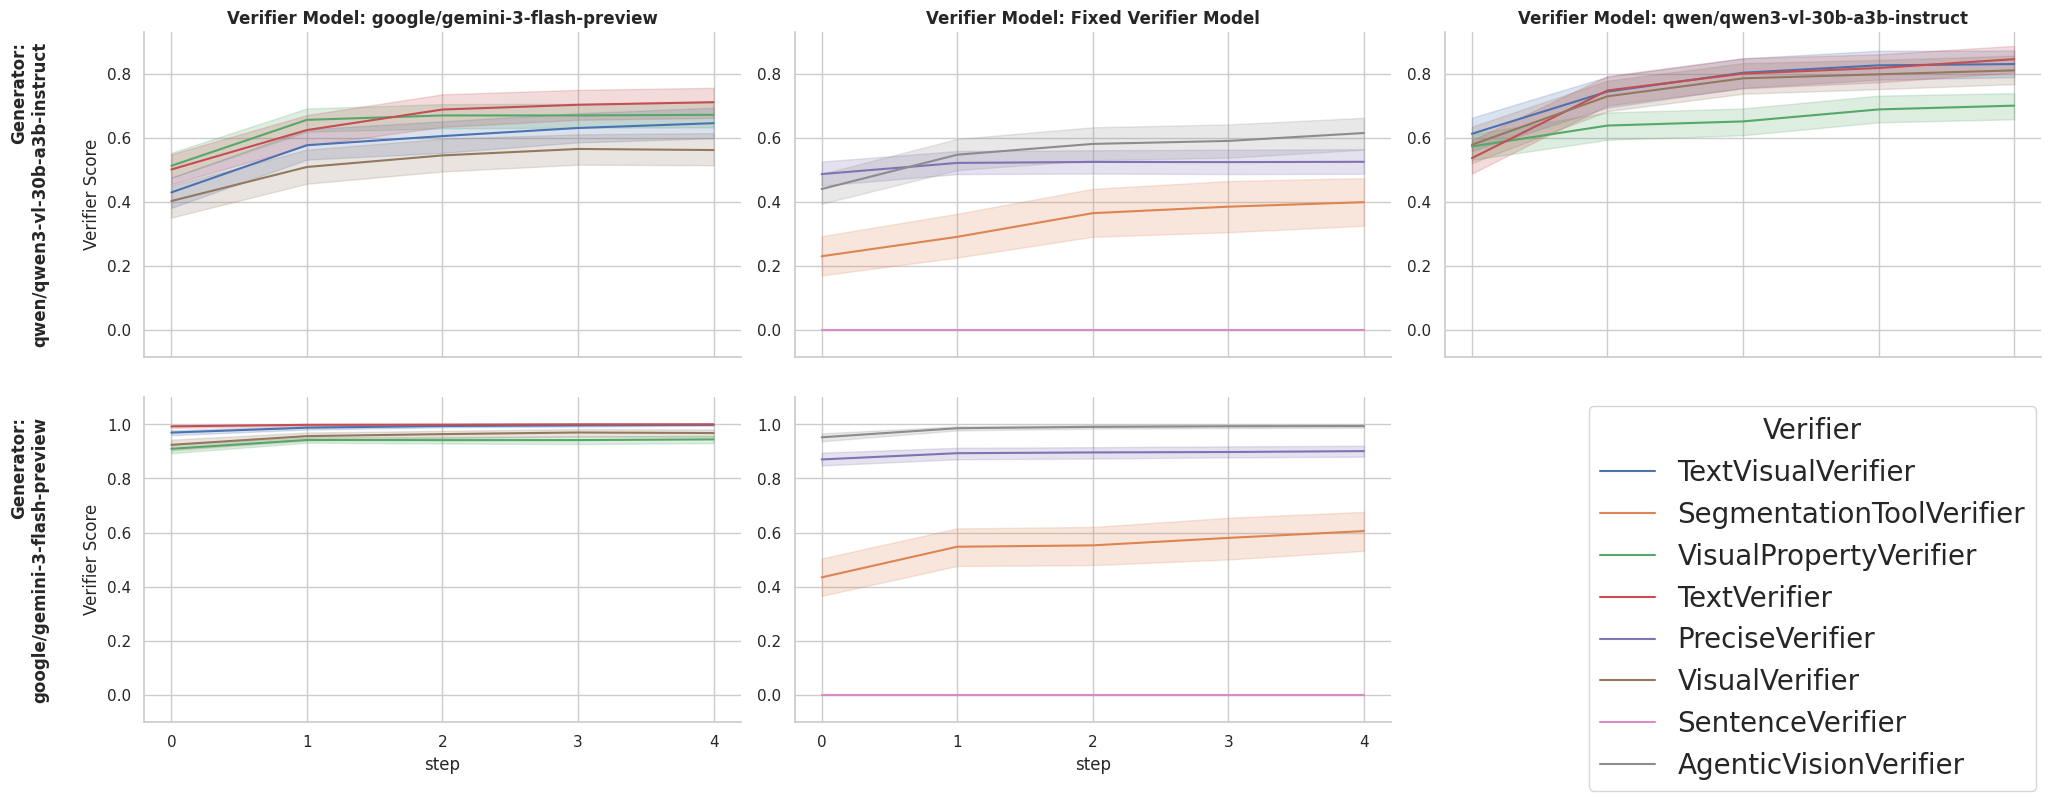}
   \caption{
       Average Verifier score per step per Verifier.
   }
    \label{figure:avg_ver_score_step}
\end{figure*}

\begin{figure}
    \centering
    \includegraphics[width=\linewidth]{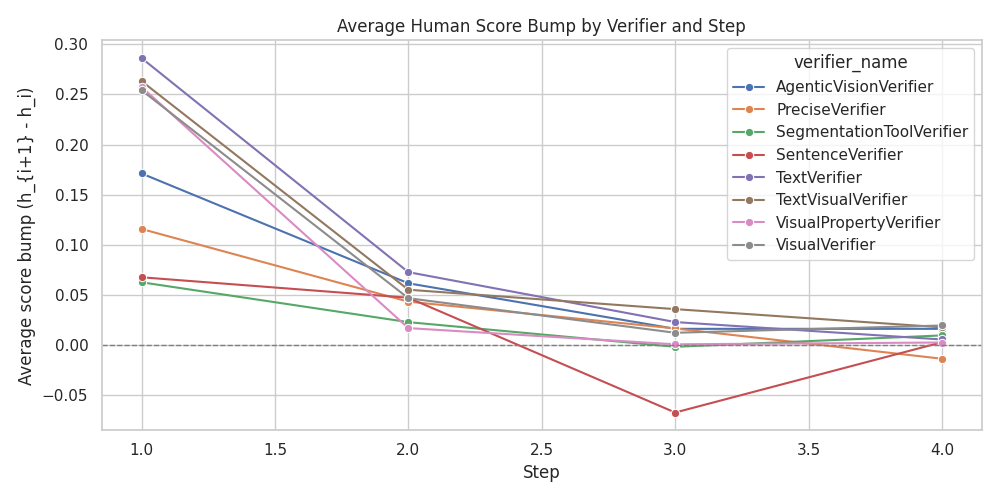}
   \caption{
       Average bump of the score per step per Verifier.
   }
    \label{figure:avg_bump_score_step}
\end{figure}
